# Supplementary material for: Limit order trading with a mean reverting reference price
Source: arXiv:1607.00454 source file (2016-11-14)
Supplement: Supplementary file 1 [file appendix_lehalle.tex]

\section{Asymptotic analysis in Gueant, Lehalle, and Fernandez-Tapia \cite{InventoryRisk}}
For completeness, we state the results of the asymptotic analysis in Gueant, Lehalle, and Fernandez-Tapia \cite{InventoryRisk}.

Consider the Avellaneda and Stoikov model 
\begin{equation}
\begin{cases}
dQ_{t} = dQ^{b}_{t} - dQ_{t}^{a} \\
dX_{t} = \left(S_{t} + \delta^{a}_{t}\right) dQ_{t}^{a} - \left(S_{t} - \delta^{b}_{t}\right)dQ_{t}^{b}\\
dS_{t} = \sigma dB_{t}\\
Q^{b}_{t}\sim \text{Poi}\left(Ae^{-\kappa \delta^{b}_{t}}\right)\\
Q^{a}_{t}\sim \text{Poi}\left(Ae^{-\kappa\delta^{a}_{t}}\right)\\
\displaystyle\sup_{\delta^{a}, \delta^{b}}E\left[-e^{- \gamma\left(X_{T} + S_{T}Q_{T}\right)}\right].
\end{cases}
\end{equation}
with a finite inventory space $\{-Q, \cdots, Q\}$. The value function is defined as
\begin{equation}
u\left(t, q, x, s\right) =\displaystyle\sup_{\delta^{a}, \delta^{b}}E\left(-e^{-\gamma W_{T}} | Q_{t} = q, X_{t} = x, S_{t} = s\right),
\end{equation}
and the HJB equations for value function are:

For $|q| < Q$,
\begin{equation}
\begin{split}
0=u_{t}& + \frac{\sigma^{2}}{2} u_{ss} + \displaystyle\max_{\delta^{a}, \delta^{b}}\left\{\vphantom{Ae^{-\kappa \delta^{b}}}\right.\\
&\left[u\left(t, q - 1, x + s + \delta^{a}, s\right) - u\left(t, q , x, s\right) \right]Ae^{-\kappa \delta^{a}} +\\
&\left. \left[u\left(t, q + 1, x - s + \delta^{b}, s\right) - u\left(t, q , x, s\right) \right]Ae^{-\kappa \delta^{b}}\right\}
\end{split}
\end{equation}

For $q = Q$,
\begin{equation}
0=u_{t} + \frac{\sigma^{2}}{2} u_{ss} + \displaystyle\max_{\delta^{a}}\left\{\vphantom{Ae^{-\kappa \delta^{b}}}\left[u\left(t, q - 1, x + s + \delta^{a}, s\right) - u\left(t, q , x, s\right) \right]Ae^{-\kappa \delta^{a}} \right\}
\end{equation}

For $q = -Q$,
\begin{equation}
\begin{split}
0=u_{t} + \frac{\sigma^{2}}{2} u_{ss} + \displaystyle\max_{\delta^{b}}\left\{\vphantom{Ae^{-\kappa \delta^{b}}} \left[u\left(t, q + 1, x - s + \delta^{b}, s\right) - u\left(t, q , x, s\right) \right]Ae^{-\kappa \delta^{b}}\right\}
\end{split}
\end{equation}
with the terminal condition:
\begin{equation}
u\left(T, q, x, s\right) = -e^{-\gamma\left(x + qs\right)},\quad\forall q\in\{-Q, \cdots, Q\}.
\end{equation}
The optimal spreads are given by
\begin{equation}
\begin{split}
\delta^{b*}\left(t,q\right)&  = \frac{1}{\kappa}\log\left(\frac{v\left(t,q\right)}{v\left(t, q+1\right)}\right) + \frac{1}{\gamma}\log\left(1 + \frac{\gamma}{\kappa}\right)\quad q\neq Q\\
\delta^{a*}\left(t,q\right)  &= \frac{1}{\kappa}\log\left(\frac{v\left(t,q\right)}{v\left(t, q-1\right)}\right) + \frac{1}{\gamma}\log\left(1 + \frac{\gamma}{\kappa}\right)\quad q\neq Q,
\end{split}
\end{equation}
where $v\left(t, q\right)$ is an ansatz satisfying
\begin{equation}
u(t, x, q, s) = -e^{-\gamma\left(x + qs\right)}v\left(t,q\right)^{-\frac{\gamma}{\kappa}}.
\end{equation}
The asymptotic result is that 
\begin{equation}
\begin{split}
\lim_{T\rightarrow\infty}\delta^{b*}\left(0, q\right) &= \frac{1}{\gamma}\log\left(1 + \frac{\gamma}{\kappa}\right) + \frac{1}{\kappa}\log\left(\frac{f^{0}_{q}}{f^{0}_{q + 1}}\right)\\
\lim_{T\rightarrow\infty}\delta^{a*}\left(0, q\right) &=\frac{1}{\gamma}\log\left(1 + \frac{\gamma}{\kappa}\right) + \frac{1}{\kappa}\log\left(\frac{f^{0}_{q}}{f^{0}_{q - 1}}\right)
\end{split}
\end{equation}
where $f^{0}\in \mathbb{R}^{2Q + 1}$ is an eigenvector corresponding to the smallest eigenvalue of the matrix $M$ defined by
\[\begin{bmatrix}
\alpha Q^{2}&-\eta&0&\cdots&\cdots&\cdots &0 \\
-\eta&\alpha (Q-1)^{2} &-\eta&0&\ddots&\ddots &\vdots \\
\vdots & \ddots & \ddots & \ddots&\ddots&\ddots&\vdots\\
0&\ddots&\ddots&0& -\eta&\alpha (Q-1)^{2} &-\eta\\
0&\cdots&\cdots&\cdots&0&-\eta&\alpha Q^{2}
\end{bmatrix}\]
 with $\alpha = \frac{\kappa}{2}\gamma\sigma^{2}$ and $\eta = A\left( 1 + \frac{\gamma}{\kappa}\right)^{-\left(1 + \frac{\kappa}{\gamma}\right)}$. We refer to Theorem 1 and Theorem 2 in \cite{InventoryRisk} for more detail.
